# Supplementary material for: Learning to See Low-Light Images via Feature Domain Adaptation
Source: arXiv:2312.06723 source file (2023-12-20)
Supplement: Supplementary file 1 [file X_suppl.tex]

\clearpage
\setcounter{page}{1}
\maketitlesupplementary

\section{More Quantitative and Qualitative Results}
\textbf{Quantitative Results.} We have processed SID-Sony using dark shading correction \cite{feng2023learnability} to reduce the effect of noise to obtain the SID-Sony-DSC dataset. We further evaluate our method on the SID-Sony-DSC dataset. Quantitative results are shown in Tab. \ref{sota_DSC}. Compared to previous methods, our method significantly outperforms.
%%%%%%%%%%%%%%%%%%%%%%%%%%%%%%%%%%%%%%%%%%%%%%%%%%%%%%%%%%%%%%%%%%%%%%%%
\begin{table*}[htp]
    \centering
    \caption{Quantitative results of RAW-based LLIE methods on the SID-Sony-DSC \cite{chen2018learning, feng2023learnability} datasets. The best result is in red \textbf{{\color{red}bold}} whereas the second best one is in blue {\color{blue}\underline{underlined}}. Metrics with $\uparrow$ and $\downarrow$ denote higher, better, and lower, respectively.}
        \begin{tabular}{clcccccc}
            \hline
            \multirow{2}{*}{Category} & \multirow{2}{*}{Method} & \multirow{2}{*}{FLOPS} & \multirow{2}{*}{\#Parm} & \multicolumn{4}{c}{Sony-DSC\cite{chen2018learning}}  \\  
            \cline{5-8}
            &     &  &     &  PSNR$\uparrow$  & SSIM$\uparrow$ & $\Delta E$$\downarrow$  & LPIPS$\downarrow$ \\  
            \hline      
            \multirow{5}{*}{Single-Stage} 
            & \multicolumn{1}{l}{LLPackNet \cite{Lamba_Balaji_Mitra_2020}}   &7.2G  &1.2M   &29.21	&0.788	&6.914	&0.1818  \\
            & \multicolumn{1}{l}{IRT \cite{Lamba_Mitra_2021}}  &5.2G    & 0.8M    &29.35	&0.786	&6.914	&0.1772 \\
            & \multicolumn{1}{l}{DID \cite{maharjan2019improving}}   & 669.2G & 2.5M   &29.61	&0.794	 &6.986  &0.1709  \\
            & \multicolumn{1}{l}{SGN \cite{gu2019self}}   &75.5G   &19.2M   &29.69	&0.796	&6.739	&0.1727  \\
            & \multicolumn{1}{l}{SID \cite{chen2018learning}}   &48.5G & 7.7M   &29.70	 &0.797  &6.789  &{\color{blue}\underline{0.1671}}  \\              
            \hline
            \multirow{3}{*}{Multi-Stage} & \multicolumn{1}{l}{LDC \cite{xu2020learning}}     &124.1G    &8.6M    &30.73	&0.799	&5.967	&0.1693  \\
            & \multicolumn{1}{l}{MCR \cite{dong2022abandoning}}  &90.5G     &15.0M    &30.85	&{\color{blue}\underline{0.801}}	&5.896	&\textbf{{\color{red}0.1661}}  \\
            & \multicolumn{1}{l}{DNF \cite{jin2023dnf}}   &57.0G   &2.8M    &{\color{blue}\underline{30.94}}	&\textbf{{\color{red}0.803}}	&{\color{blue}\underline{5.751}}	&0.1682 \\
            \hline
            \multirow{1}{*}{\textbf{Single-Stage}} & \multicolumn{1}{l}{\textbf{Ours}}   &34.0G   &1.7M    &\textbf{{\color{red}31.17}}	&\textbf{{\color{red}0.803}}	&\textbf{{\color{red}5.682}}	&0.1678  \\
            \hline
    \end{tabular} 
    \label{sota_DSC}
\end{table*}

%%%%%%%%%%%%%%%%%%%%%%%%%%%%%%%%%%%%%%%%%%%%%%%%%%%%%%%%%%%%%%%%%%%%%%%%
%%%%%%%%%%%%%%%%%%%%%%%%%%%%%%%%%%%%%%%%%%%%%%%%%%%%%%%%%%%%%%%%%%%%%%%%
\begin{table}[htp]
    \centering
    \caption{Quantitative results of RAW-based LLIE methods on the MCR-Mono \cite{dong2022abandoning} datasets. The best result is in red \textbf{{\color{red}bold}} whereas the second best one is in blue {\color{blue}\underline{underlined}}.}
        \begin{tabular}{clcccccc}
            \hline
            \multirow{2}{*}{Category} & \multirow{2}{*}{Method} & \multicolumn{2}{c}{MCR-Mono\cite{dong2022abandoning}}  \\  
            \cline{5-8}
            &     &   PSNR$\uparrow$  & SSIM$\uparrow$ \\  
            \hline      
            \multirow{5}{*}{Single-Stage} 
            & \multicolumn{1}{l}{IRT \cite{Lamba_Mitra_2021}}  &25.74	&0.851	\\
            & \multicolumn{1}{l}{DID \cite{maharjan2019improving}}   &26.16	&0.888	 \\
            & \multicolumn{1}{l}{SGN \cite{gu2019self}}  &29.29	&0.882	\\
            & \multicolumn{1}{l}{SID \cite{chen2018learning}}   &29.00	 &0.906  \\              
            \hline
            \multirow{3}{*}{Multi-Stage} & \multicolumn{1}{l}{LDC \cite{xu2020learning}}     &29.36	&0.904	 \\
            & \multicolumn{1}{l}{MCR \cite{dong2022abandoning}}  &31.69	& 0.908\\
            & \multicolumn{1}{l}{DNF \cite{jin2023dnf}}    &{\color{blue}\underline{32.00}}	&{\color{blue}\underline{0.915}} \\
            \hline
            \multirow{1}{*}{\textbf{Single-Stage}} & \multicolumn{1}{l}{\textbf{Ours}}   &\textbf{{\color{red}32.33}}	&\textbf{{\color{red}0.917}} \\
            \hline
    \end{tabular} 
    \label{sota_mcr}
\end{table}

%%%%%%%%%%%%%%%%%%%%%%%%%%%%%%%%%%%%%%%%%%%%%%%%%%%%%%%%%%%%%%%%%%%%%%%%
\begin{figure*}
    \centering	   
    \centering{\includegraphics[width=17.35cm]{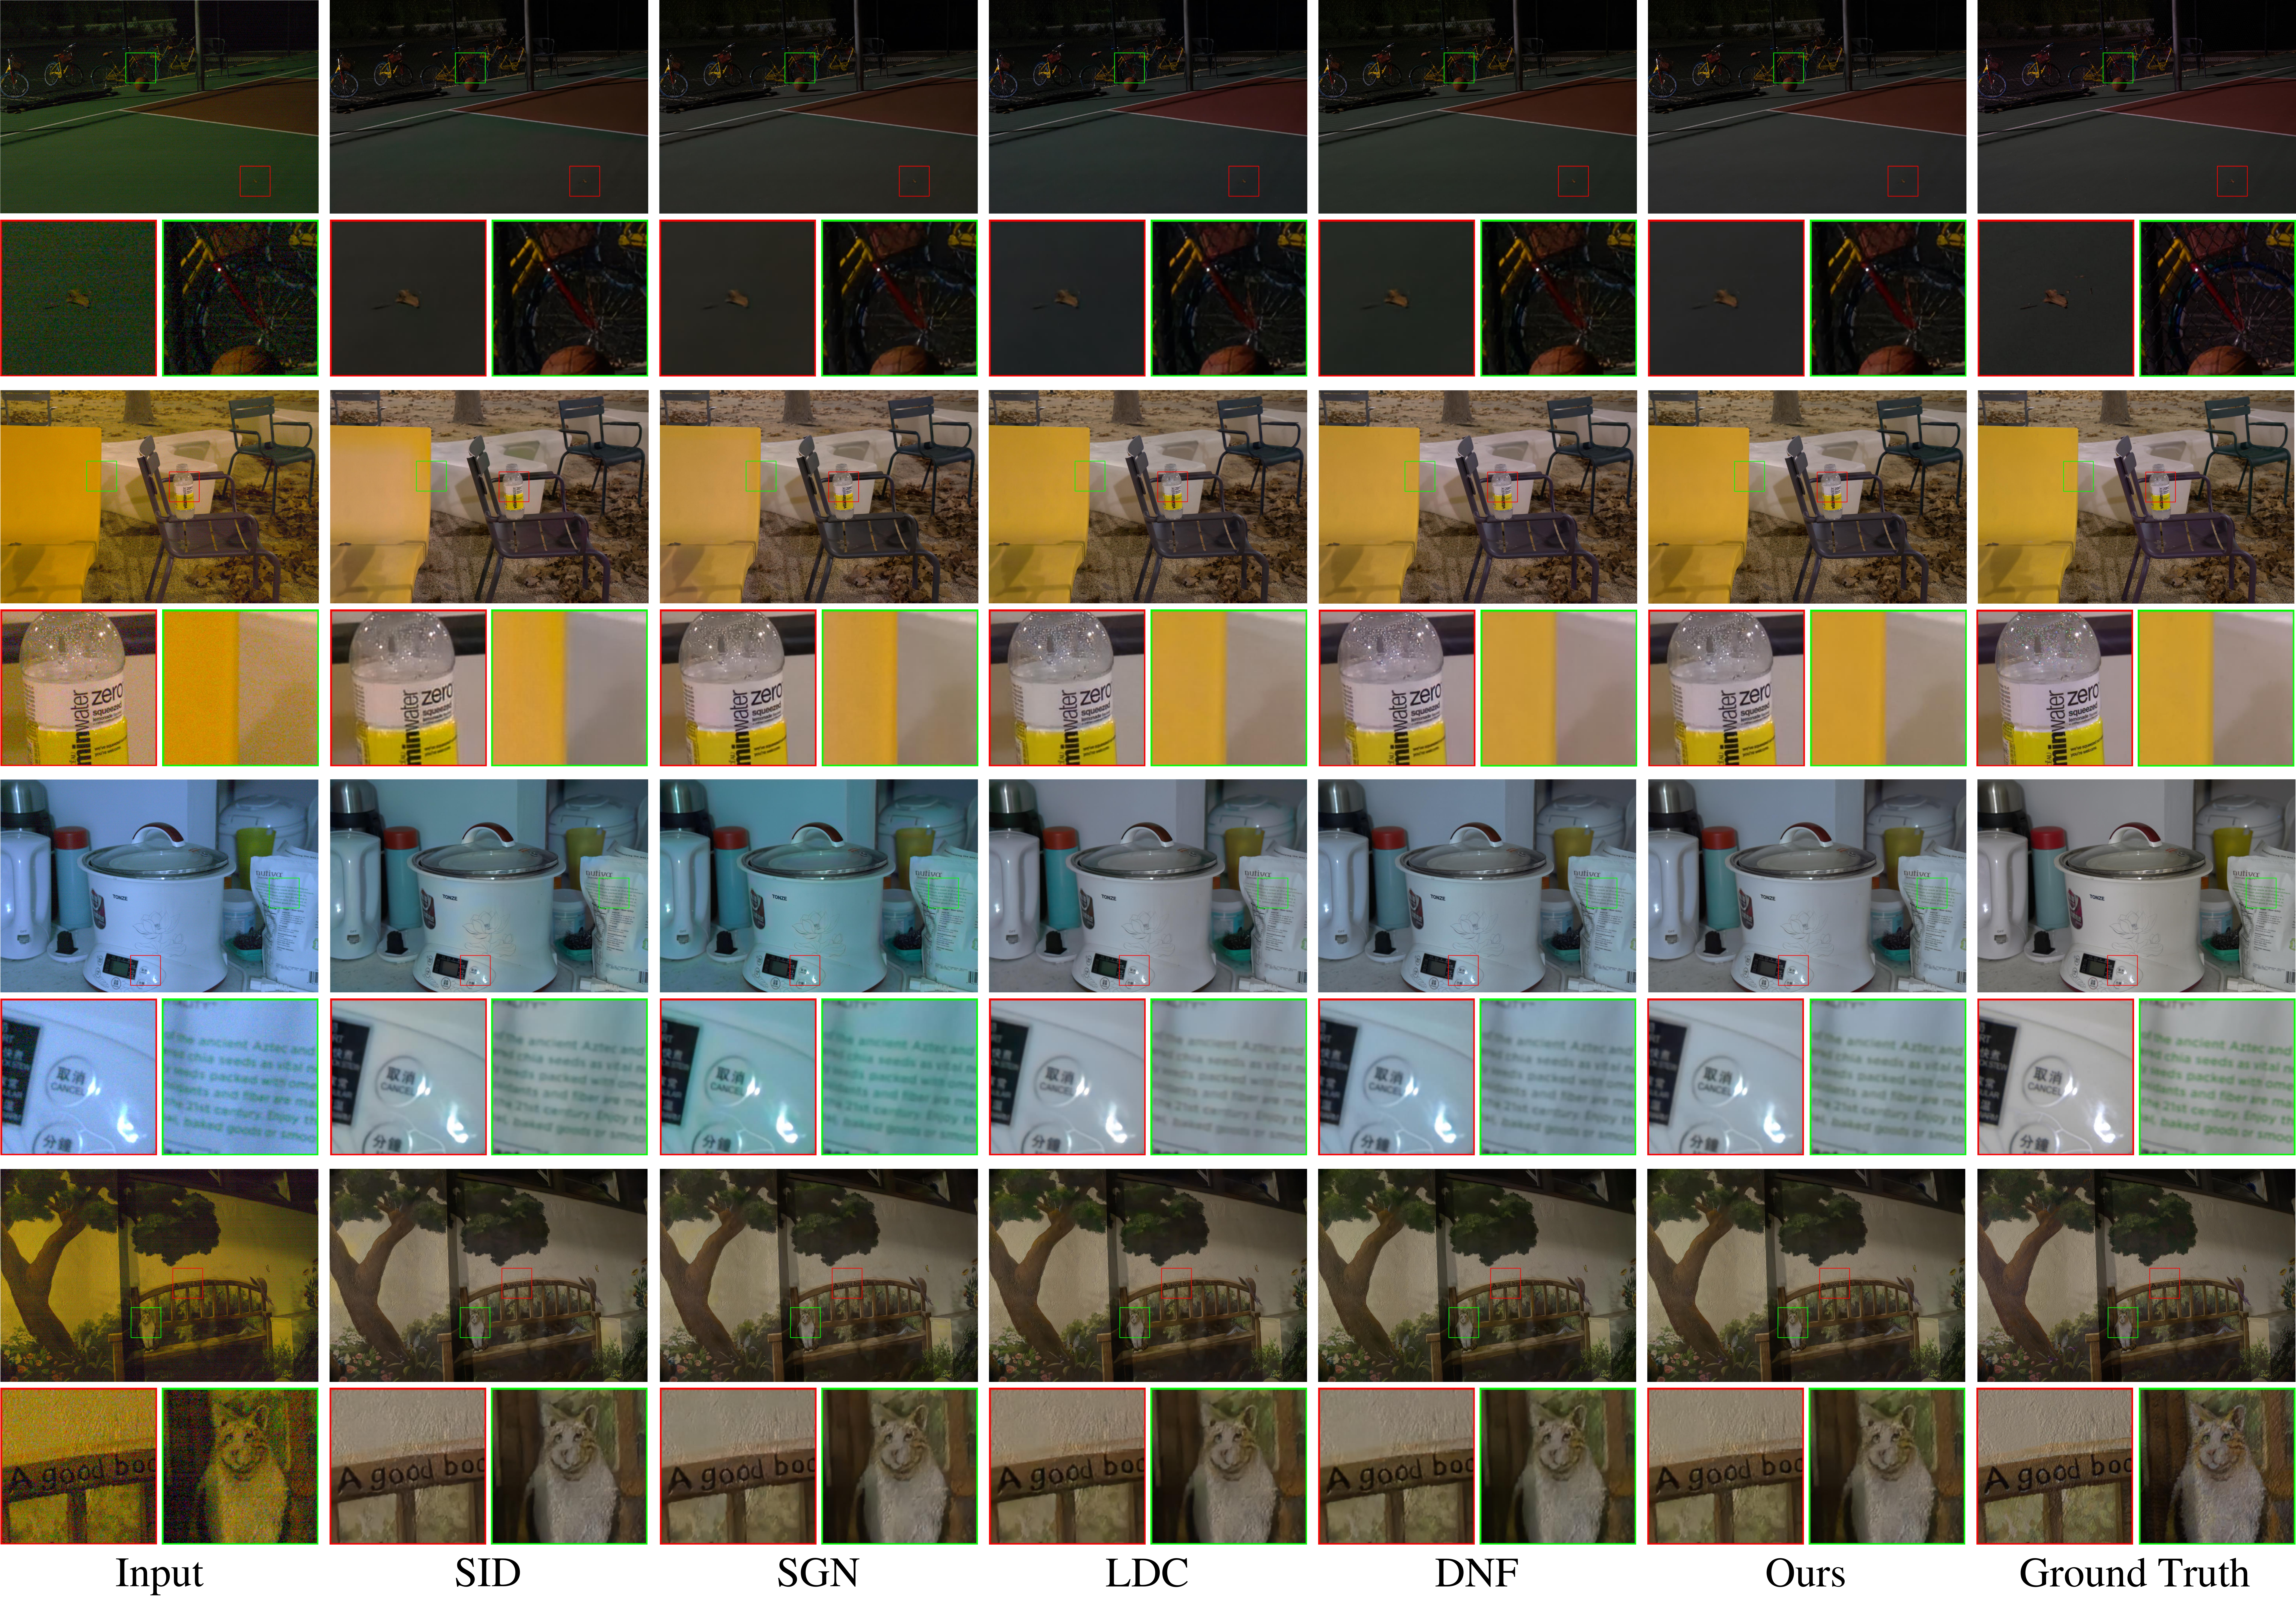}}  
    \caption {Visual comparisons between our FDANet and the state-of-the-art methods on the SID-Sony dataset (Zoom-in for best view).}
    \label{visual_sid_sup}
\end{figure*}

\begin{figure*}
    \centering	   
    \centering{\includegraphics[width=17.35cm]{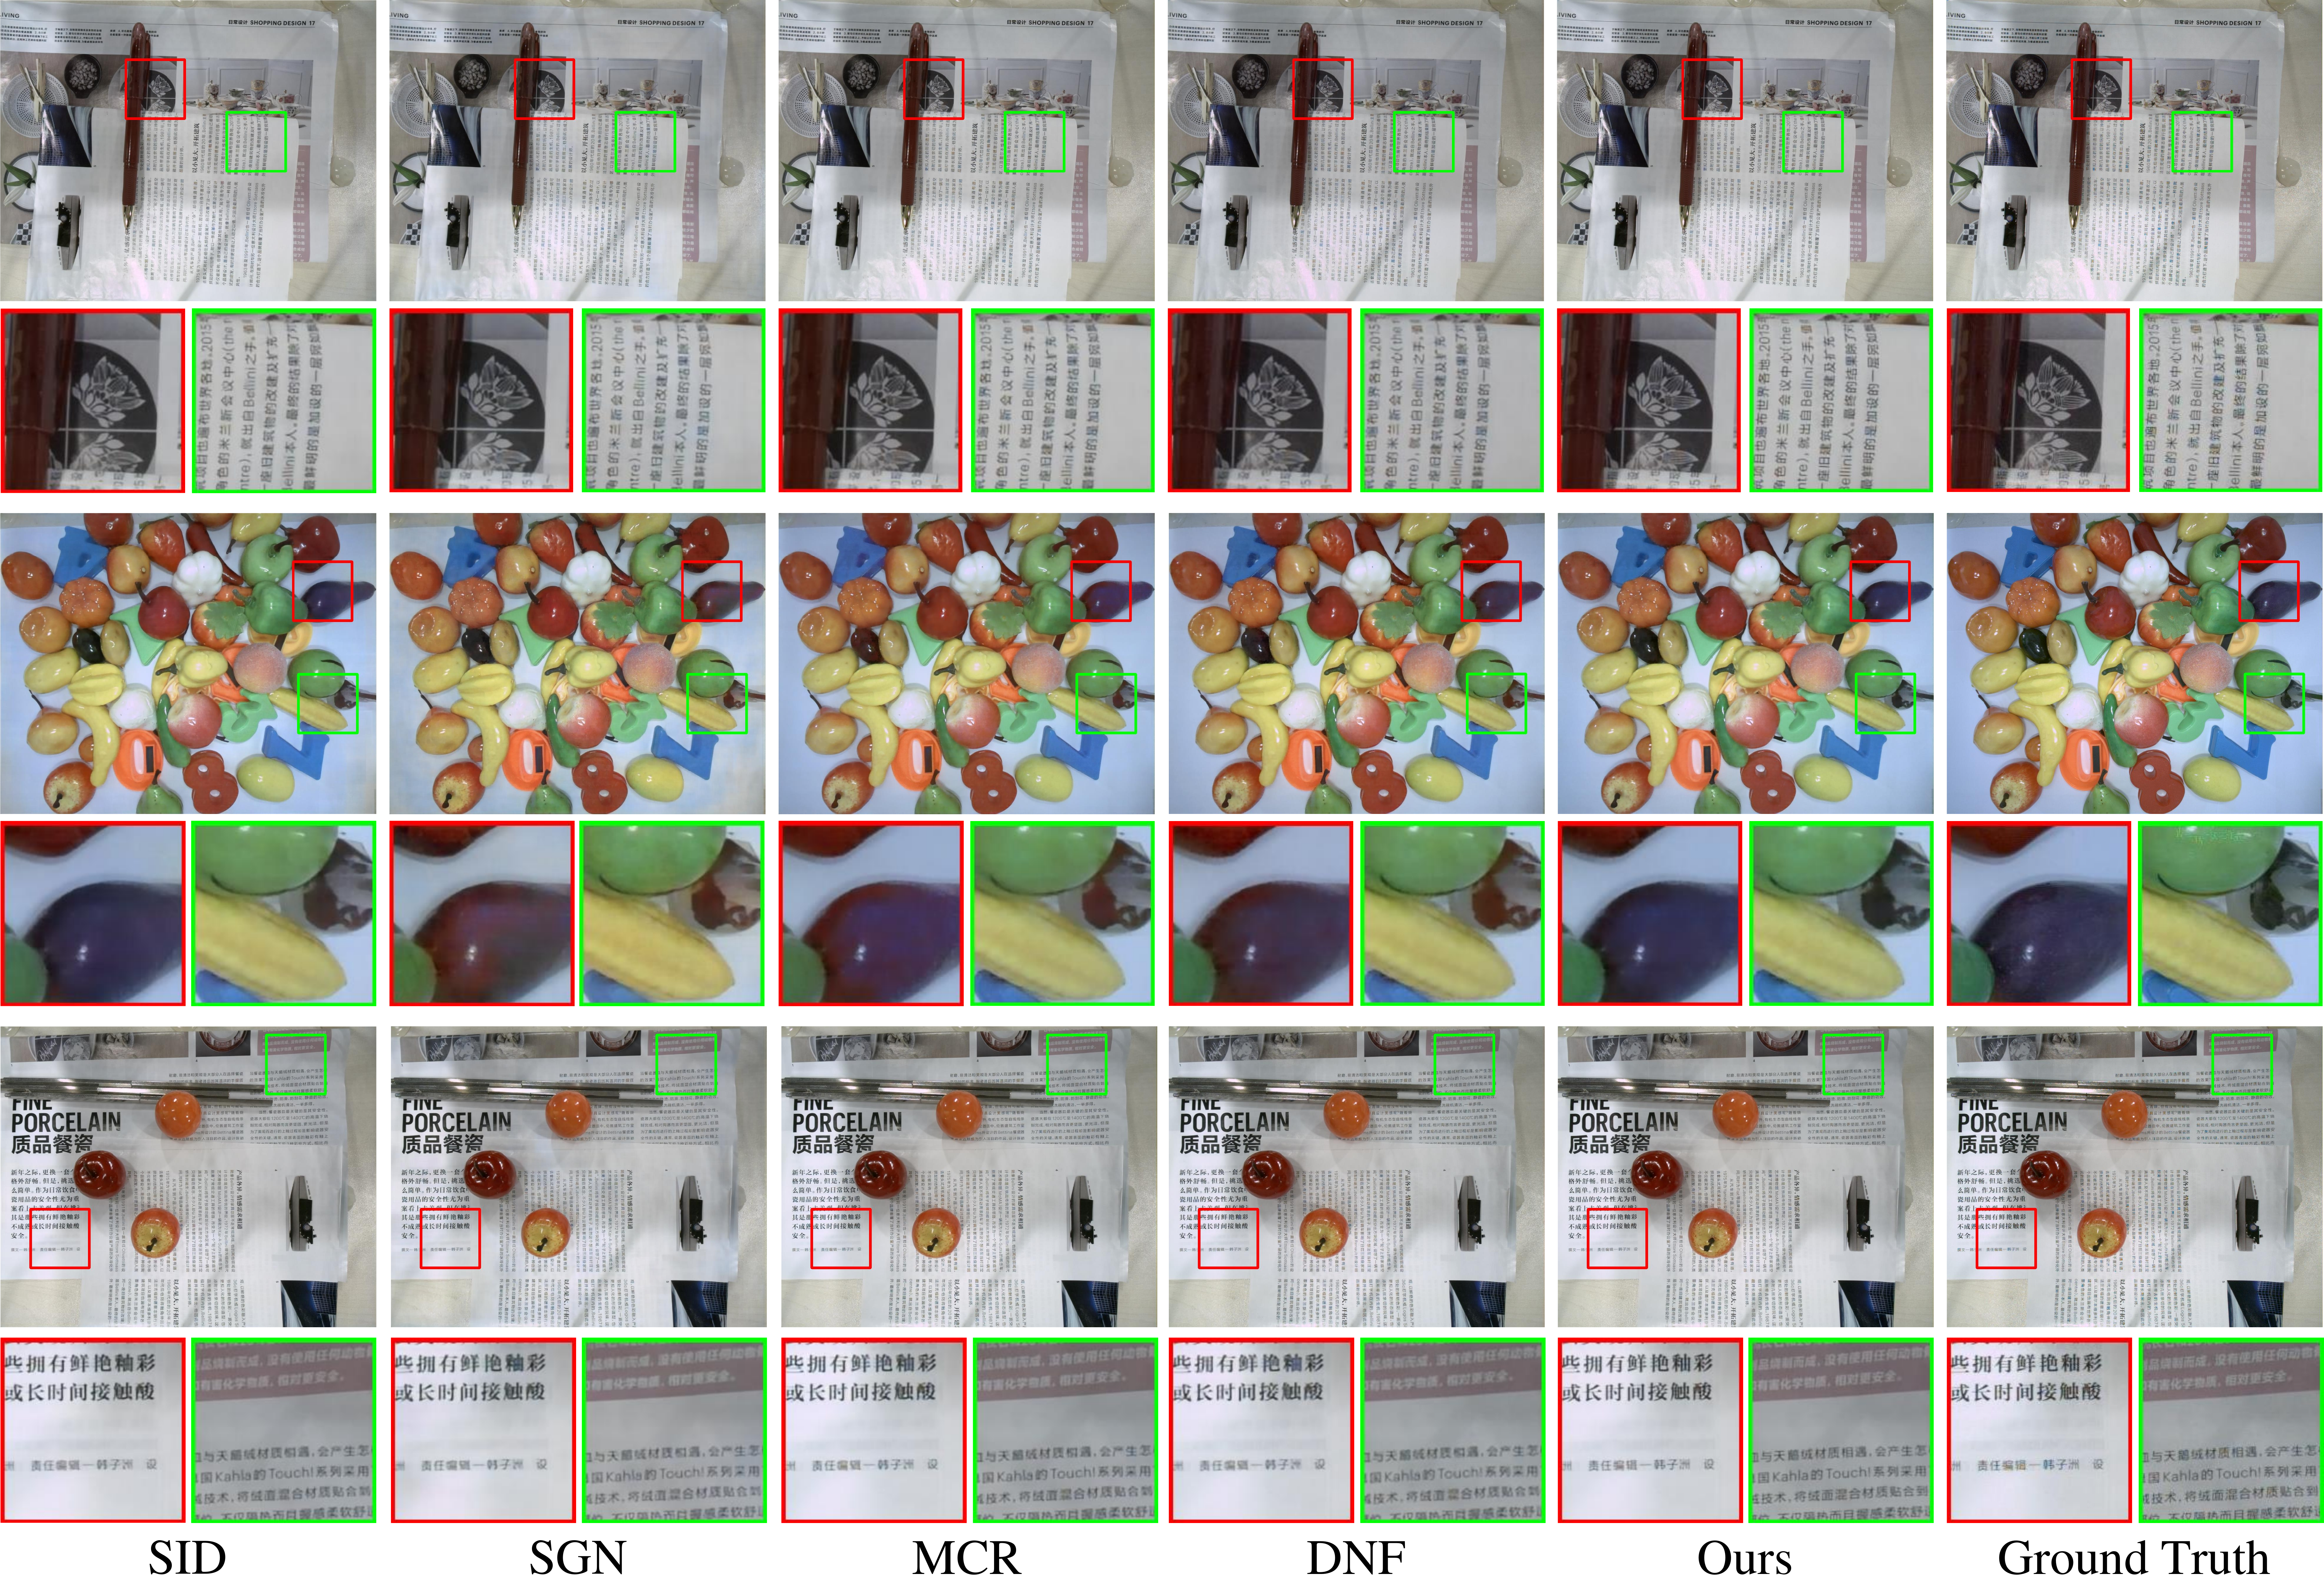}}  
    \caption {Visual comparisons between our FDANet and the state-of-the-art methods on the MCR dataset (Zoom-in for best view).}
    \label{visual_sid_sup}
\end{figure*}
